# Supplementary material for: Kohn-Sham decomposition in real-time time-dependent density-functional theory: An efficient tool for analyzing plasmonic excitations
Source: arXiv:1703.02824 ancillary file (2017-03-08)
Supplement: Supplementary file 1 [file supplement.pdf]

# Supplemental Material for “Kohn–Sham decomposition in real-time time-dependent density-functional theory: An efficient tool for analyzing plasmonic excitations”

T. P. Rossi,[1,*] M. Kuisma,[2,3] M. J. Puska,[1] R. M. Nieminen,[1] and P. Erhart[2]

[1] *COMP Centre of Excellence, Department of Applied Physics, Aalto University School of Science, Espoo, Finland*

[2] *Department of Physics, Chalmers University of Technology, Gothenburg, Sweden*

[3] *Department of Chemistry, Nanoscience Center, University of Jyväskylä, Jyväskylä, Finland*

* tuomas.rossi@alumni.aalto.fi

## Additional transition contribution maps for $Ag_{55}$

We present here the transition contribution maps (TCMs) for the $Ag_{55}$ nanoparticle from $\omega = 3.65\,\mathrm{eV}$ to $\omega = 4.30\,\mathrm{eV}$ in steps of $0.01\,\mathrm{eV}$. All TCMs use the same color scale. See the main text for the description of the plots.

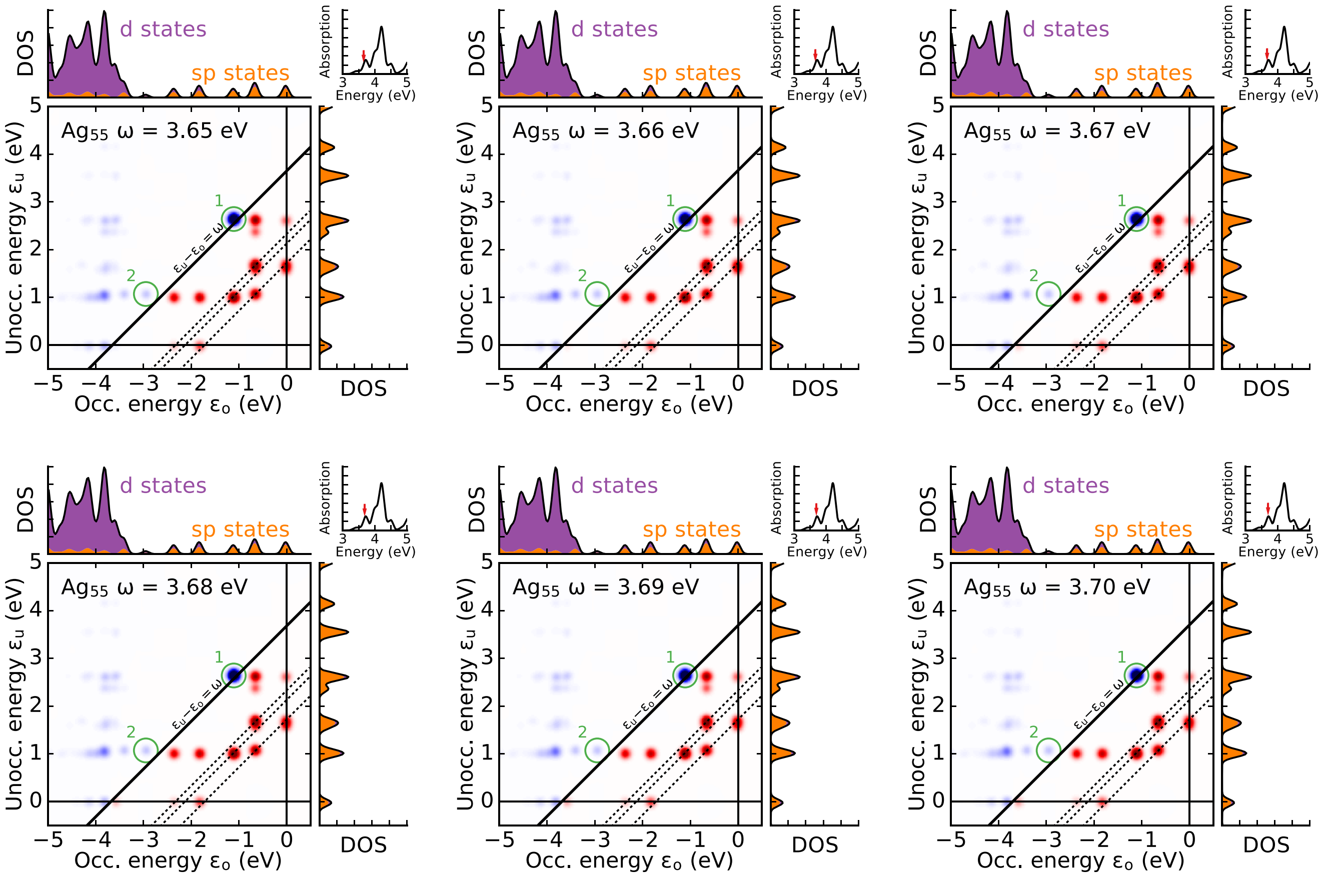

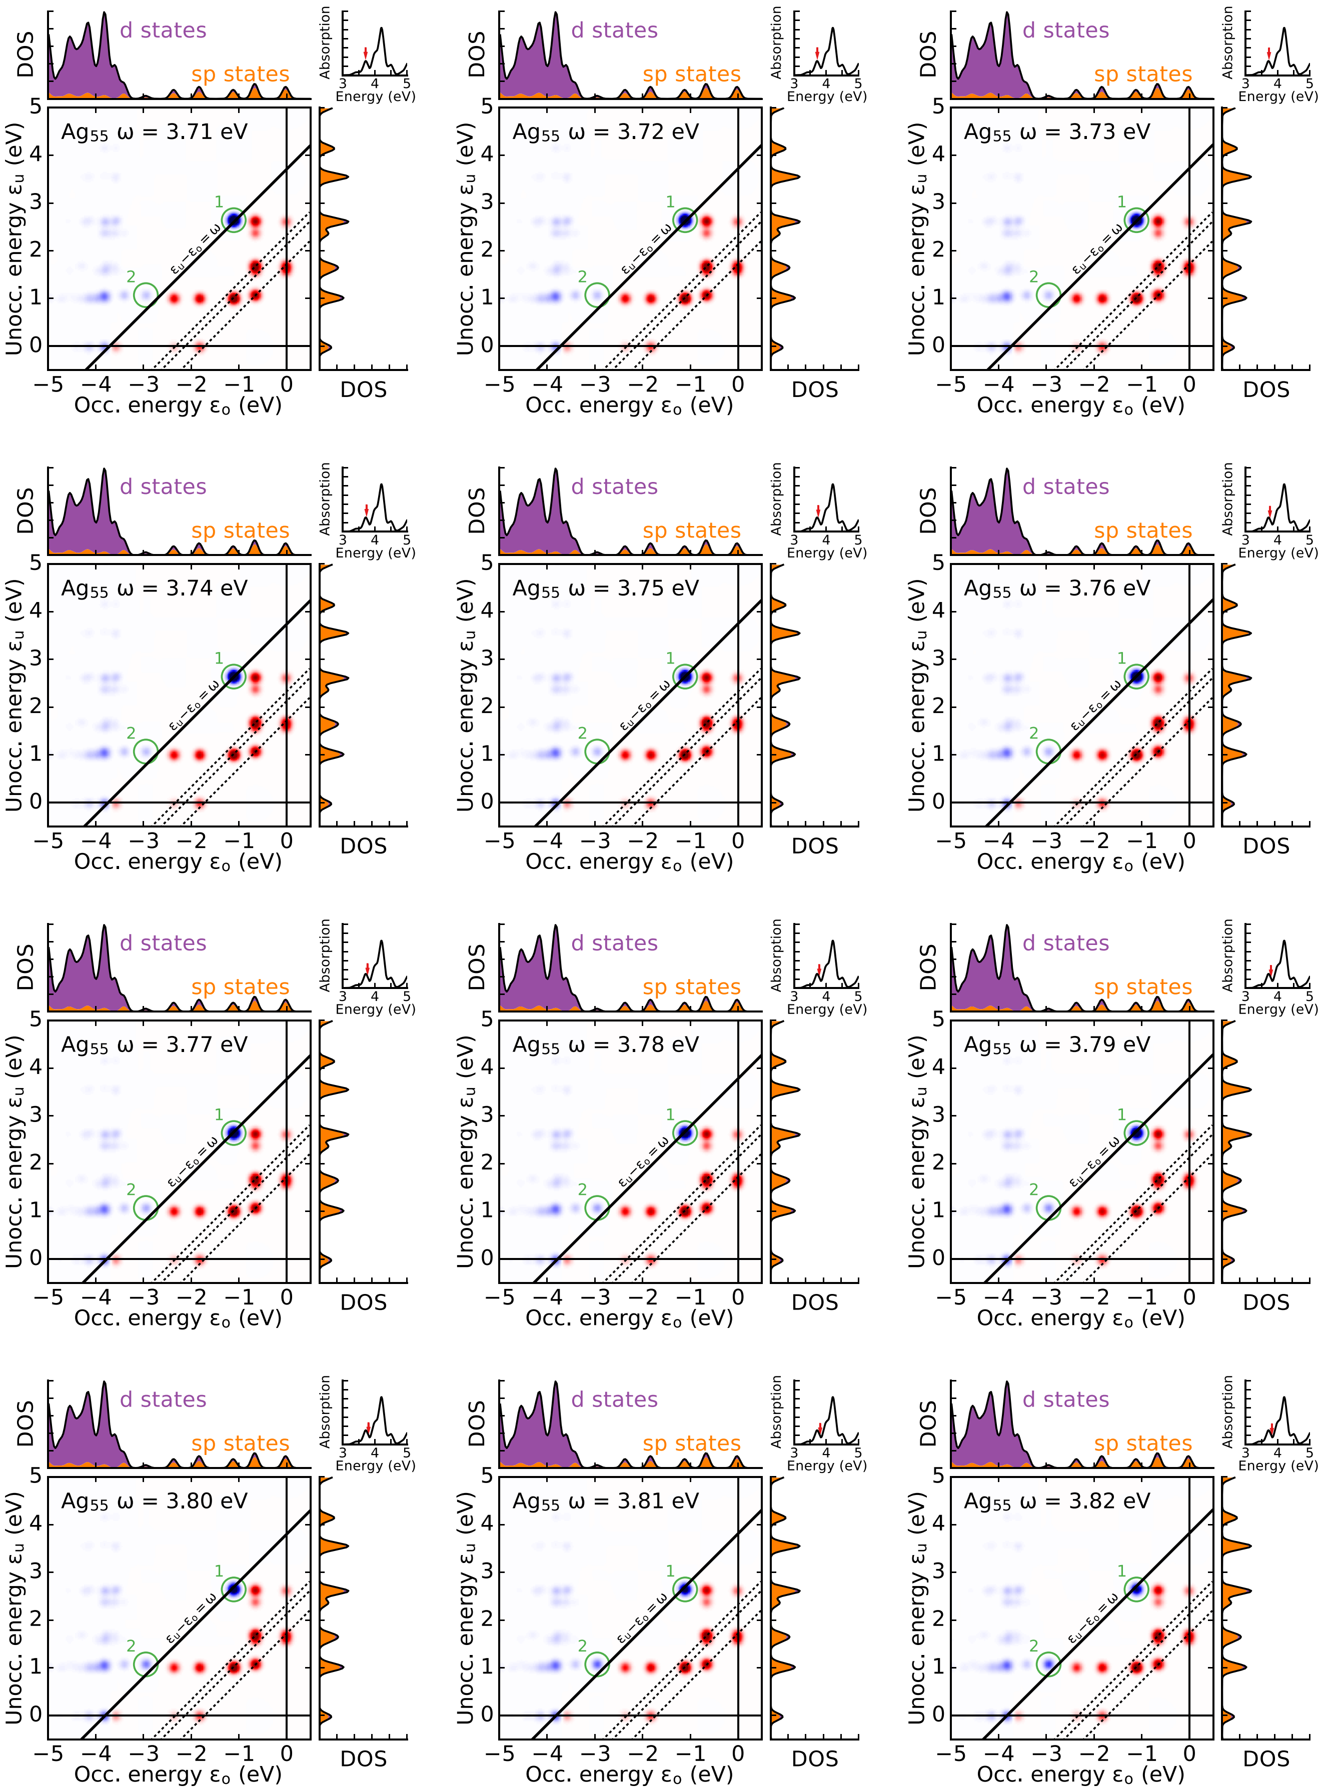

Ag55 ω = 3.71 eV
Ag55 ω = 3.72 eV
Ag55 ω = 3.73 eV
Ag55 ω = 3.74 eV
Ag55 ω = 3.75 eV
Ag55 ω = 3.76 eV
Ag55 ω = 3.77 eV
Ag55 ω = 3.78 eV
Ag55 ω = 3.79 eV
Ag55 ω = 3.80 eV
Ag55 ω = 3.81 eV
Ag55 ω = 3.82 eV
d states
sp states
DOS
Absorption
Energy (eV)
Unocc. energy εu (eV)
Occ. energy εo (eV)
εu−εo = ω

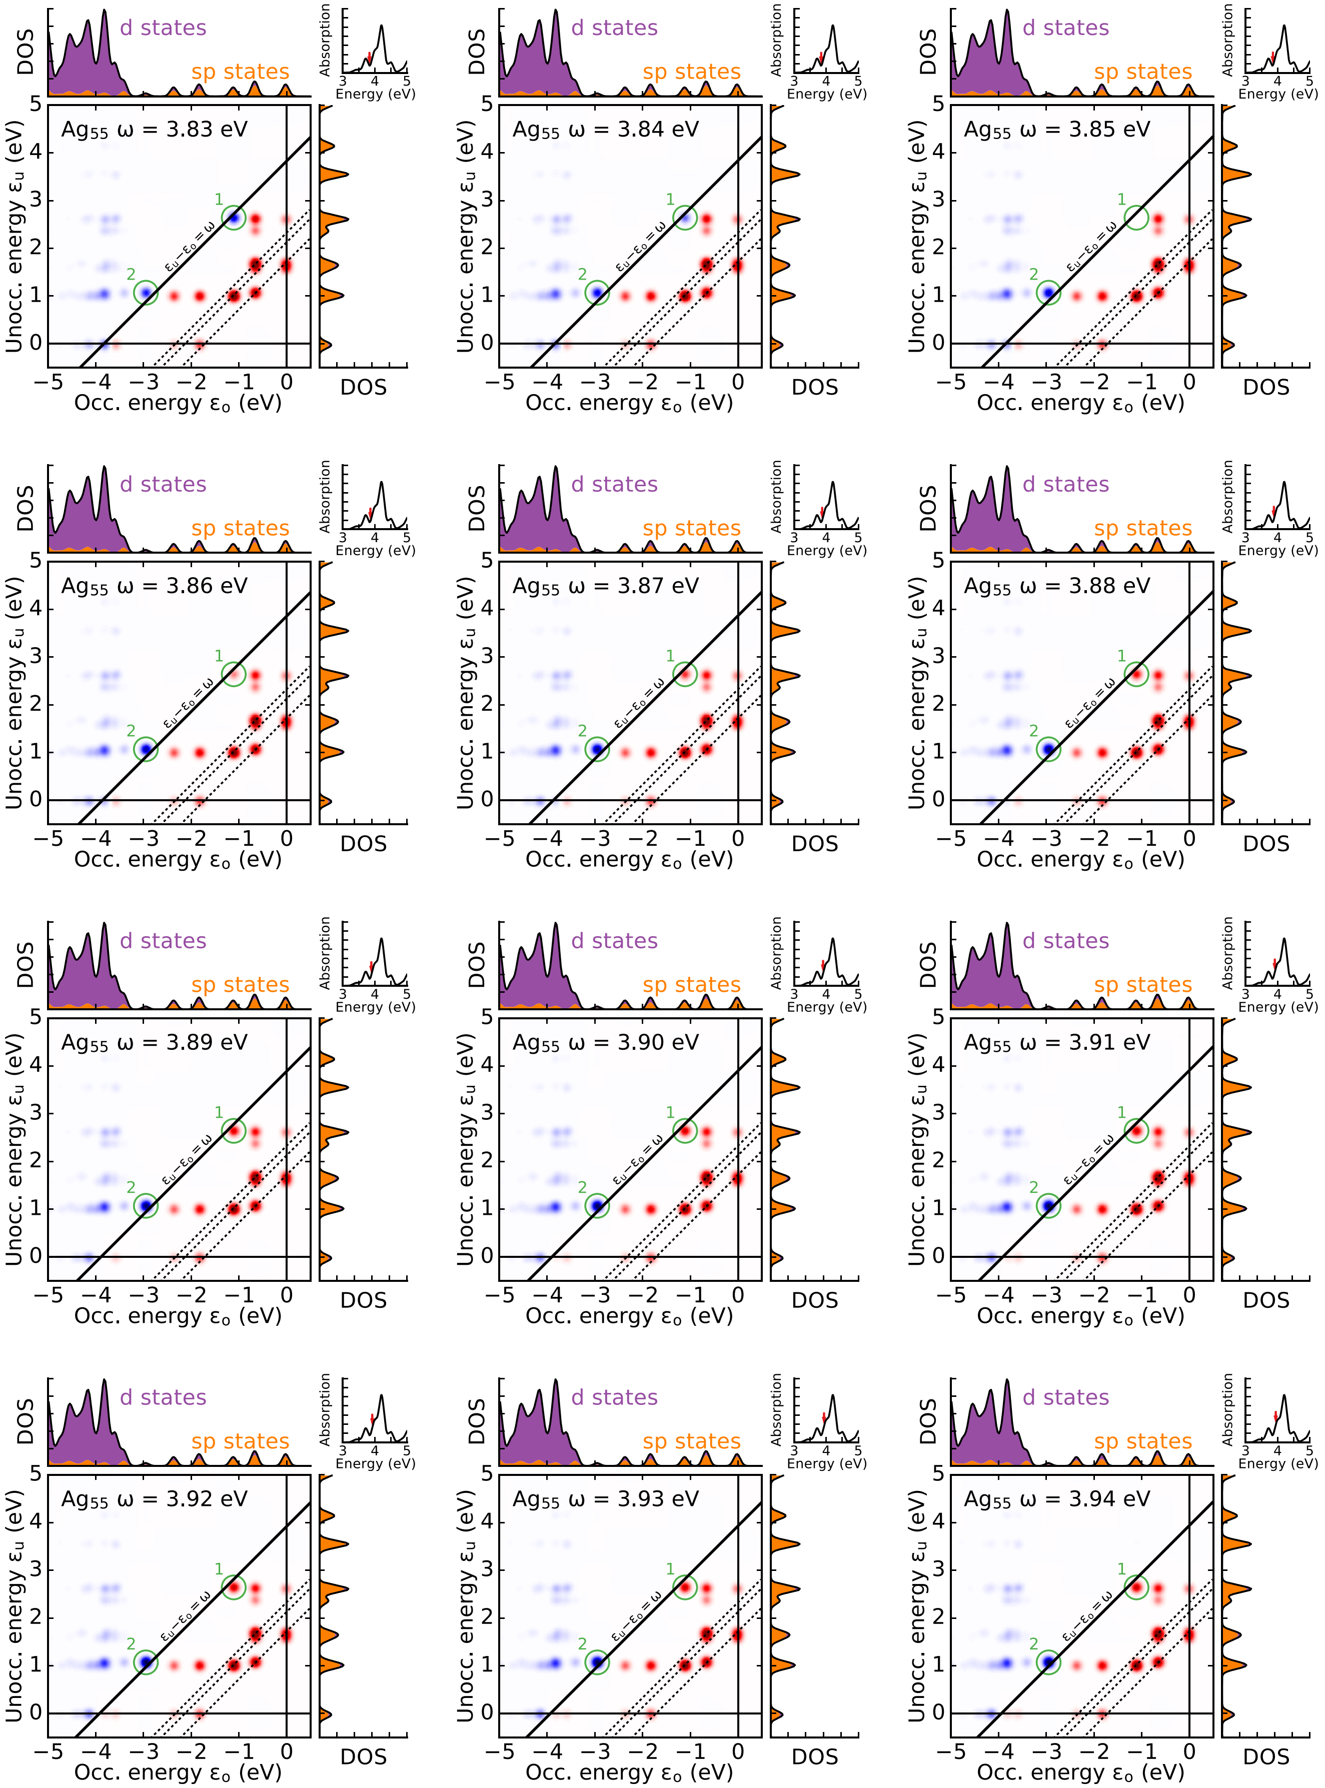

DOS
d states
sp states
Absorption
Energy (eV)
Ag55 ω = 3.83 eV
Ag55 ω = 3.84 eV
Ag55 ω = 3.85 eV
Ag55 ω = 3.86 eV
Ag55 ω = 3.87 eV
Ag55 ω = 3.88 eV
Ag55 ω = 3.89 eV
Ag55 ω = 3.90 eV
Ag55 ω = 3.91 eV
Ag55 ω = 3.92 eV
Ag55 ω = 3.93 eV
Ag55 ω = 3.94 eV
εu−εo = ω
Unocc. energy εu (eV)
Occ. energy εo (eV)

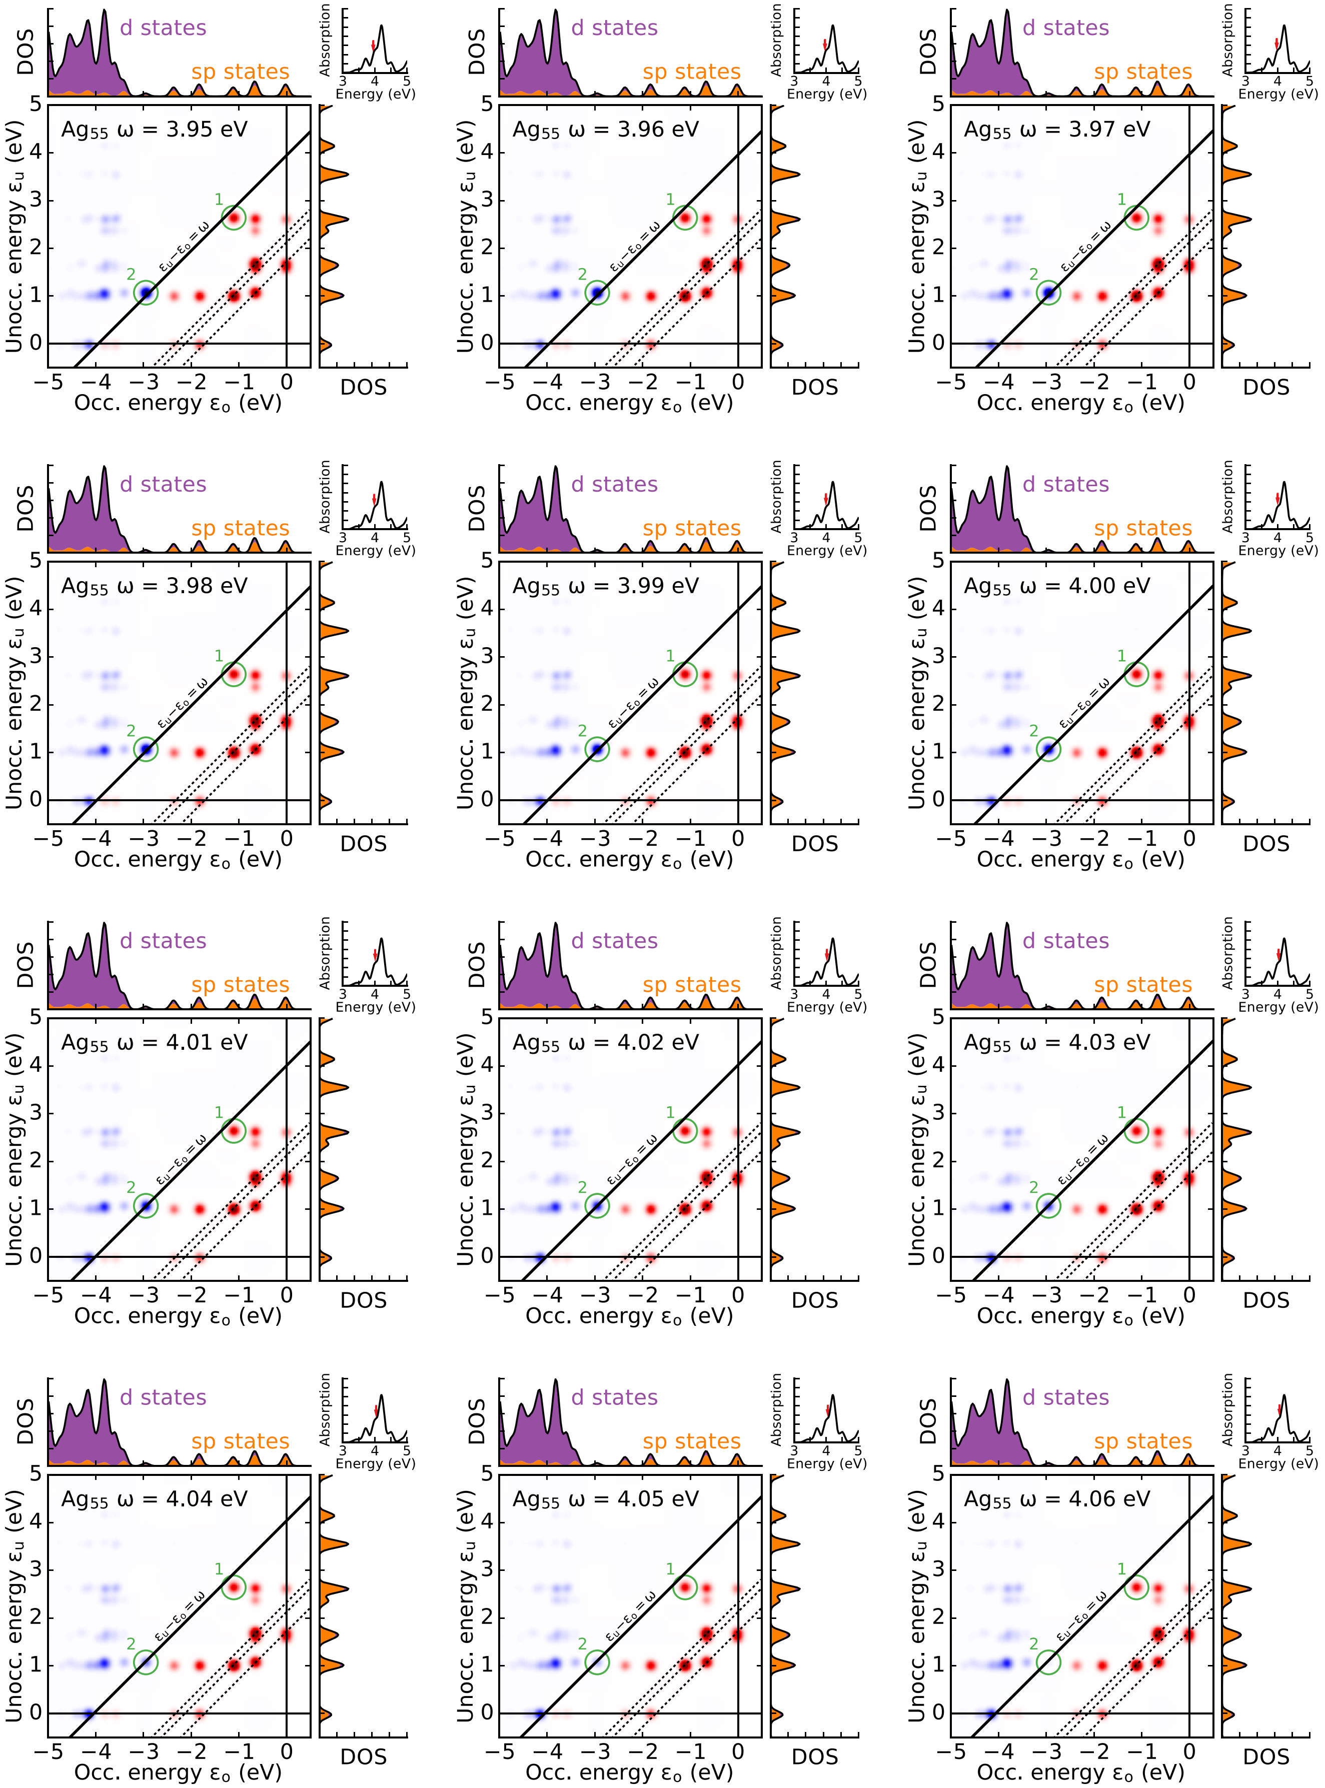

d states
sp states
DOS
Absorption
Energy (eV)
Ag55 ω = 3.95 eV
Ag55 ω = 3.96 eV
Ag55 ω = 3.97 eV
Ag55 ω = 3.98 eV
Ag55 ω = 3.99 eV
Ag55 ω = 4.00 eV
Ag55 ω = 4.01 eV
Ag55 ω = 4.02 eV
Ag55 ω = 4.03 eV
Ag55 ω = 4.04 eV
Ag55 ω = 4.05 eV
Ag55 ω = 4.06 eV
εu−εo = ω
Unocc. energy εu (eV)
Occ. energy εo (eV)

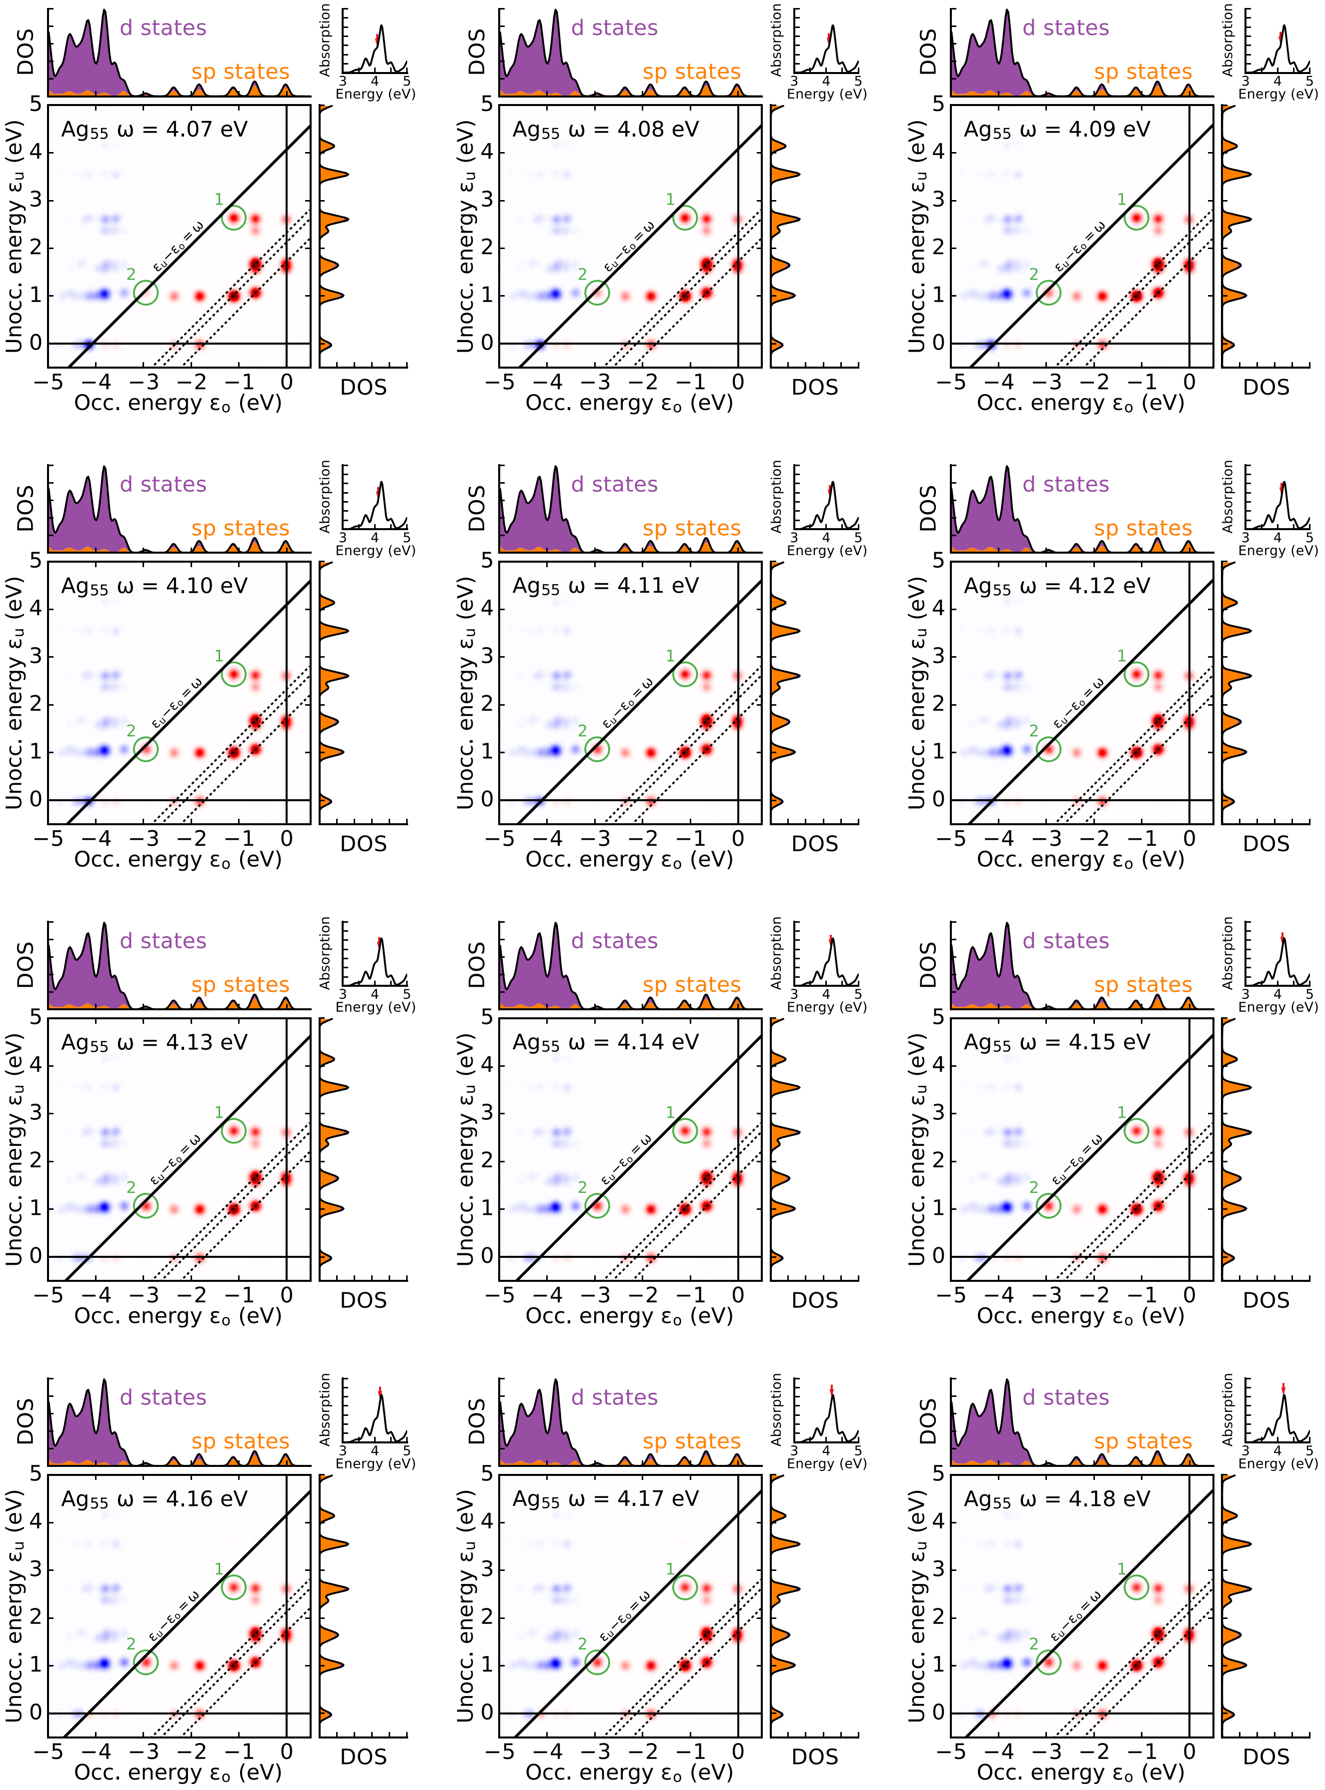

DOS
d states
sp states
Absorption
Energy (eV)
Ag$_{55}$ ω = 4.07 eV
Ag$_{55}$ ω = 4.08 eV
Ag$_{55}$ ω = 4.09 eV
Ag$_{55}$ ω = 4.10 eV
Ag$_{55}$ ω = 4.11 eV
Ag$_{55}$ ω = 4.12 eV
Ag$_{55}$ ω = 4.13 eV
Ag$_{55}$ ω = 4.14 eV
Ag$_{55}$ ω = 4.15 eV
Ag$_{55}$ ω = 4.16 eV
Ag$_{55}$ ω = 4.17 eV
Ag$_{55}$ ω = 4.18 eV
$\varepsilon_u - \varepsilon_o = \omega$
Unocc. energy $\varepsilon_u$ (eV)
Occ. energy $\varepsilon_o$ (eV)

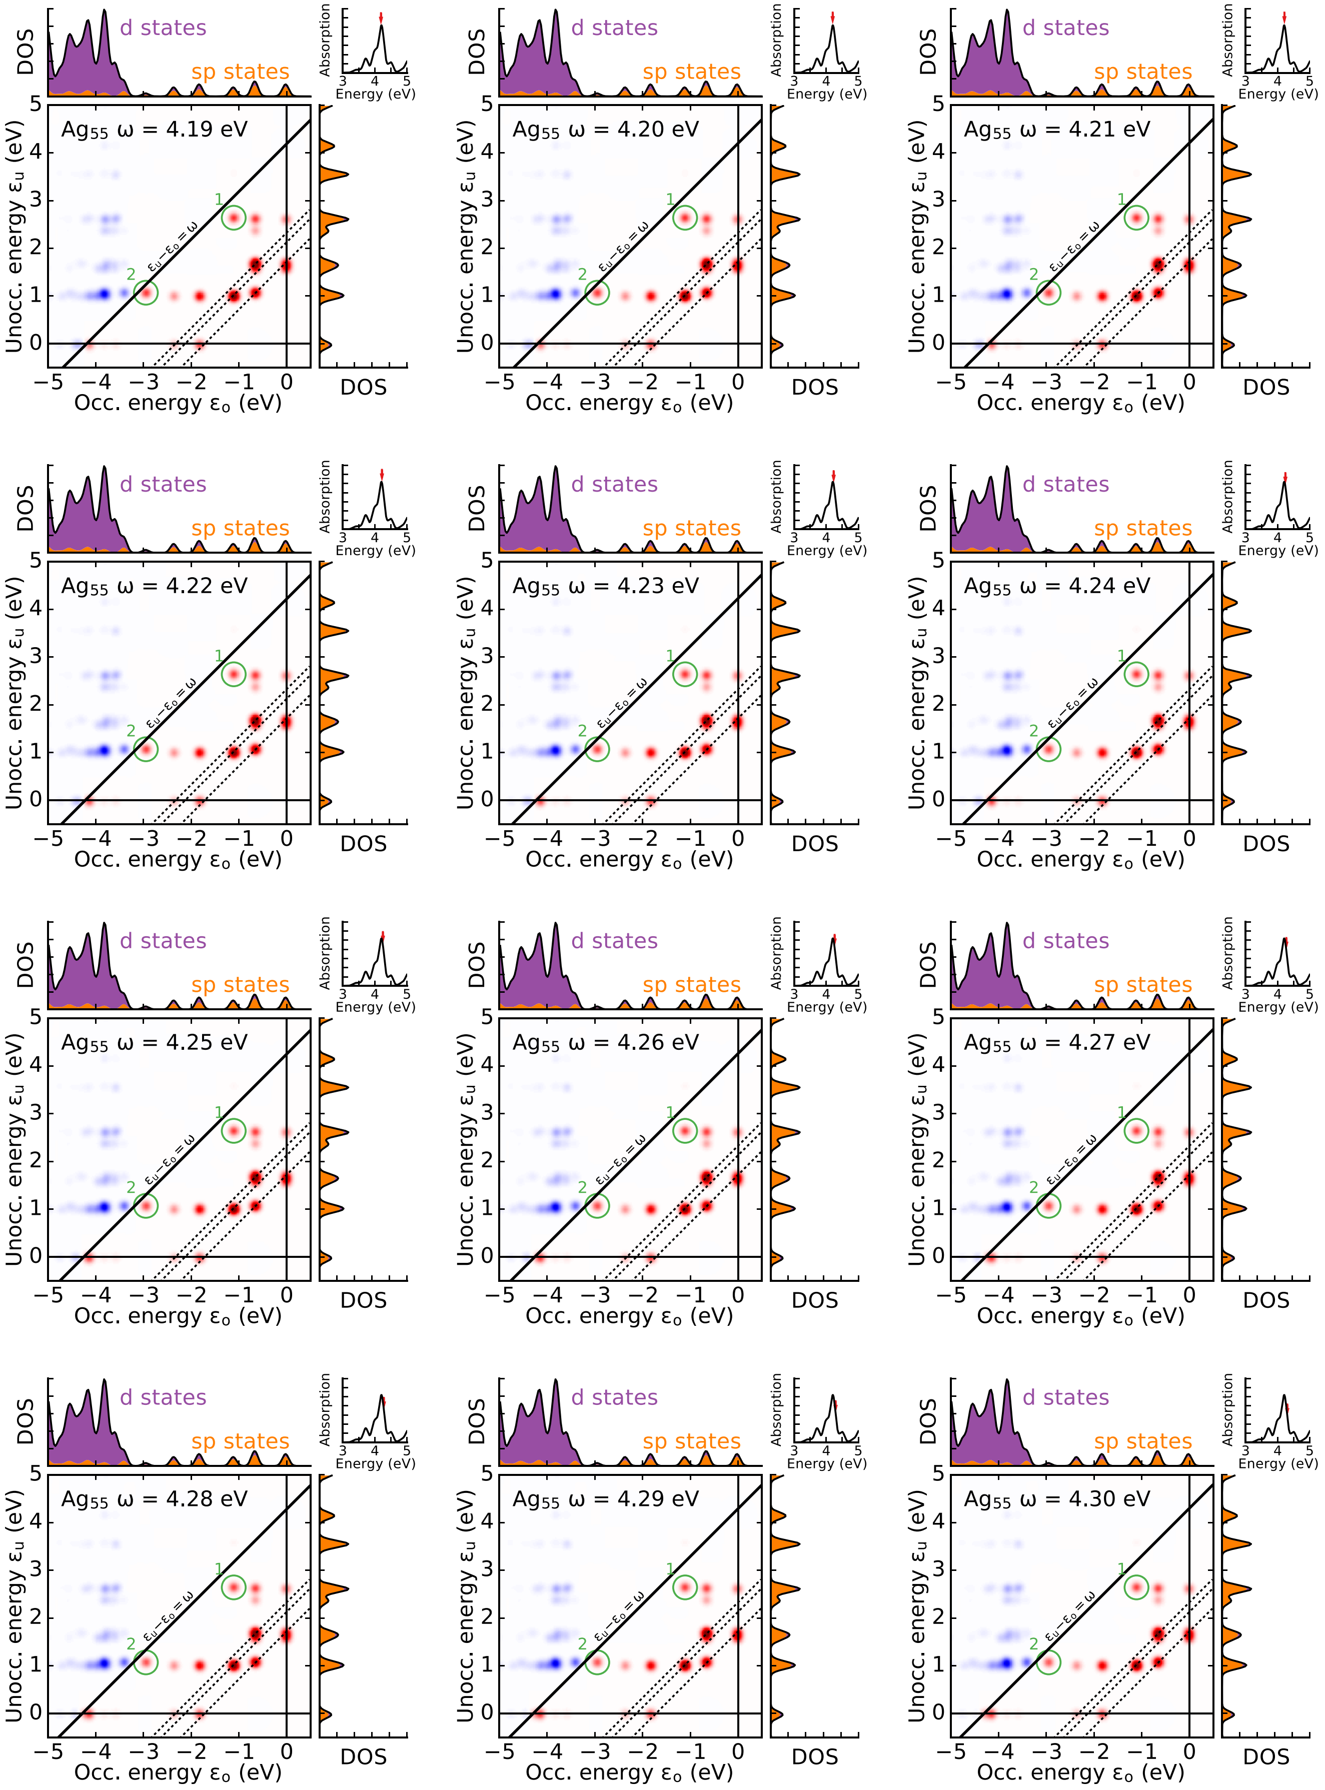
Ag55 ω = 4.19 eV
Ag55 ω = 4.20 eV
Ag55 ω = 4.21 eV
Ag55 ω = 4.22 eV
Ag55 ω = 4.23 eV
Ag55 ω = 4.24 eV
Ag55 ω = 4.25 eV
Ag55 ω = 4.26 eV
Ag55 ω = 4.27 eV
Ag55 ω = 4.28 eV
Ag55 ω = 4.29 eV
Ag55 ω = 4.30 eV
d states
sp states
DOS
Absorption
Energy (eV)
εu−εo = ω
Unocc. energy εu (eV)
Occ. energy εo (eV)
